# Supplementary material for: NextStep-1: Toward Autoregressive Image Generation with Continuous Tokens at Scale
Source: arXiv:2508.10711 source file (2025-08-18)
Supplement: Supplementary file 1 [file appendix.tex]

\newpage
\appendix
\section*{Appendix}
You may include other additional sections here.
